# Supplementary material for: Progressively-connected Light Field Network for Efficient View Synthesis
Source: arXiv:2207.04465 source file (2022-07-10)
Supplement: Supplementary file 1 [file flops.tex]

\begin{table}[htb]
    \begin{tabular}{c|c|c|c|c|c|c}
        \hline
        & ProLiF$_0$ & ProLiF$_1$ & ProLiF$_2$ & ProLiF$_3$ & ProLiF$_4$ & NeRF \\
        \hline
        FLOPs & 0.13M & 0.27M & 0.57M & 1.25M & 2.88M & 109M
    \end{tabular}
    \caption{{\bf FLOPs comparison.} }
    \label{tab:supp_flops}
\end{table}
